# Supplementary material for: SceneScript: Reconstructing Scenes With An Autoregressive Structured Language Model
Source: arXiv:2403.13064 source file (2024-03-19)
Supplement: Supplementary file 1 [file supp.tex]

\documentclass[runningheads]{llncs}

% ---------------------------------------------------------------
% Include basic ECCV package
 
% TODO REVIEW: Insert your submission number below by replacing '*****'
% TODO FINAL: Comment out the following line for the camera-ready version
\usepackage[review,year=2024,ID=7833]{eccv}
% TODO FINAL: Un-comment the following line for the camera-ready version
%\usepackage{eccv}

% OPTIONAL: Un-comment the following line for a version which is easier to read
% on small portrait-orientation screens (e.g., mobile phones, or beside other windows)
%\usepackage[mobile]{eccv}

% ---------------------------------------------------------------
% Other packages

% Commonly used abbreviations (\eg, \ie, \etc, \cf, \etal, etc.)
\usepackage{eccvabbrv}

% Include other packages here, before hyperref.
\usepackage{graphicx}
\usepackage{booktabs}
\usepackage{listings}
\usepackage{multirow}

% The "axessiblity" package can be found at: https://ctan.org/pkg/axessibility?lang=en
\usepackage[accsupp]{axessibility}  % Improves PDF readability for those with disabilities.

% ---------------------------------------------------------------
% Hyperref package

% It is strongly recommended to use hyperref, especially for the review version.
% Please disable hyperref *only* if you encounter grave issues.
% hyperref with option pagebackref eases the reviewers' job, but should be disabled for the final version.
%
% If you comment hyperref and then uncomment it, you should delete
% main.aux before re-running LaTeX.
% (Or just hit 'q' on the first LaTeX run, let it finish, and you
%  should be clear).

% TODO FINAL: Comment out the following line for the camera-ready version
\usepackage[pagebackref,breaklinks,colorlinks,citecolor=eccvblue]{hyperref}
% TODO FINAL: Un-comment the following line for the camera-ready version
%\usepackage{hyperref}

% Support for ORCID icon
\usepackage{orcidlink}

% ---------------------------------------------------------------
% structured language syntax highlighting
\lstdefinestyle{dtypestyle}{ basicstyle=\ttfamily\bfseries\color{blue} }
\lstdefinestyle{cmdstyle}{ basicstyle=\ttfamily\bfseries\color{black} }

% Define custom language
\definecolor{darkgray}{gray}{0.3}
\definecolor{darkgreen}{RGB}{50, 150, 50}
\definecolor{darkred}{RGB}{180, 50, 50}
\definecolor{darkblue}{RGB}{80, 106, 156}
\definecolor{col1}{HTML}{506A88}
\definecolor{col2}{HTML}{2E3D47}
\definecolor{col3}{HTML}{98A9B5}
\definecolor{col4}{HTML}{D19C83}
\definecolor{fom}{RGB}{0,153,139}

\lstdefinelanguage{StructuredLanguage}
{
  basicstyle=\ttfamily\bfseries,
  morekeywords={id, a_x, a_b, a_z, b_x, b_y, b_z, position_x, position_y, position_z, wall0_id, wall1_id, width, height, thickness, wall_id, pos_x, pos_y, size_x, size_y},
  keywords = [2]{string, bool, int, float},
  keywords = [3]{make_wall, make_wall_prim, make_door, make_bbox, make_prim,make_curved_wall},
  keywordstyle=\color{darkgray},
  keywordstyle=[2]\bfseries\color{blue},
  keywordstyle=[3]\bfseries\color{blue},
  sensitive=false,
  breaklines=true
}

% Define style for different types of tokens
\lstset{language=StructuredLanguage}

\begin{document}
\include{custom_commands}
% ---------------------------------------------------------------
% TODO REVIEW: Replace with your title
\title{\METHOD: Supplementary Material}

% TODO REVIEW: If the paper title is too long for the running head, you can set
% an abbreviated paper title here. If not, comment out.
\titlerunning{SceneScript}

% TODO FINAL: Replace with your author list. 
% Include the authors' OCRID for the camera-ready version, if at all possible.
\author{First Author\inst{1}\orcidlink{0000-1111-2222-3333} \and
Second Author\inst{2,3}\orcidlink{1111-2222-3333-4444} \and
Third Author\inst{3}\orcidlink{2222--3333-4444-5555}}

% TODO FINAL: Replace with an abbreviated list of authors.
\authorrunning{F.~Author et al.}
% First names are abbreviated in the running head.
% If there are more than two authors, 'et al.' is used.

% TODO FINAL: Replace with your institution list.
\institute{Princeton University, Princeton NJ 08544, USA \and
Springer Heidelberg, Tiergartenstr.~17, 69121 Heidelberg, Germany
\email{lncs@springer.com}\\
\url{http://www.springer.com/gp/computer-science/lncs} \and
ABC Institute, Rupert-Karls-University Heidelberg, Heidelberg, Germany\\
\email{\{abc,lncs\}@uni-heidelberg.de}}

\maketitle

\input{sections/suppmat}

% ---- Bibliography ----
%
% BibTeX users should specify bibliography style 'splncs04'.
% References will then be sorted and formatted in the correct style.
%
\bibliographystyle{splncs04}
\bibliography{main}

% \clearpage
% supp mat

\end{document}
